# Supplementary material for: The scale of cosmic homogeneity as a standard ruler
Source: arXiv:1810.09362 source file (2018-12-18)
Supplement: Supplementary file 1 [file Chapter_APPENDIX.tex]

\appendix

%------------------------------------------------------------------------------------------------------------------------
\section{From $\xi(r)$ to $\mathcal{N}(<r)$}\label{APP:Nr_of_xi}

The probability of finding a galaxy within a volume $dV$ around another galaxy depends on the two-point correlation function $\xi(\vec{r})$~\cite{LSS-Peebles}:
	\begin{equation}
		dP = \bar{\rho} \left[ 1 + \xi(\vec{r}) \right] dV \; .
	\end{equation}
The {counts-in-spheres} of the distribution of galaxies is then related to the correlation function:
\begin{equation}
	N(<r) = \int dP = \bar{\rho} \int \left[ 1+\xi(\vec{r'}) \right] dV \ .
\end{equation}
Assuming $\xi(\vec{r})=\xi(r)$ we get:
\begin{equation}\label{count_in_spheres_app}
	N(<r)  =  4\pi\bar{\rho} \int^{r}_{o} \left[ 1+\xi(r') \right] r'^{2} dr' \ .
\end{equation}
For the random homogeneous distribution, $\displaystyle	N_{R}(<r) = \bar{\rho} \frac{4\pi}{3}r^{3}$,
so
\begin{equation}
	\mathcal{N}(<r) = \frac{N(<r)}{N_R(<r)} = \frac{3}{r^3}\int^{r}_{o} \left[ 1+\xi(r') \right] r'^{2} dr' = 1 + \frac{3}{r^3}\int^{r}_{o} \xi(r') r'^{2} dr' \ .
\end{equation}

%------------------------------------------------------------------------------------------------------------------------
\section{Choice of estimator for ${\mathcal{N}}(<r)$} \label{subsec:Choice}

In section~\ref{subsect:Estimators}, we consider two estimators for ${\mathcal{N}}(<r)$, defined by equations (\ref{eq:lau}) and (\ref{eq:Counts}). We compute ${\mathcal{N}}(<r)$ and the resulting ${\mathcal{D}}_2(r)$ with the two estimators for the 1000 QPM mock catalogues. Figure \ref{fig:difference-Nest} compares the mean of the 1000 mocks to the $\Lambda$CDM model. The result with the cor estimator are much closer to the $\Lambda$CDM model. 

\begin{figure}[h!]
	\centering
	\includegraphics[width=0.48\linewidth, keepaspectratio]{images/JMJC_diff_all_nr.pdf}
	\includegraphics[width=0.48\linewidth, keepaspectratio]{images/JMJC_diff_all_d2.pdf}
	\caption{\label{fig:difference-Nest} 
Top: the scaled counts-in-spheres, $\mathcal{N}(<r)$, (left) and the fractal correlation dimension, $\mathcal{D}_{2}(r)$, (right) for matter distribution, with lau (black) and cor (blue) estimators, compared to $\Lambda$CDM model (red).
Bottom: the ratio to $\Lambda$CDM model for both estimator.}
\end{figure}

%------------------------------------------------------------------------------------------------------------------------
\section{Tuning errors in RSD Analysis}\label{APP:RSD-robust}

\begin{figure}[h!]
	\centering
	\includegraphics[width=.49\linewidth, keepaspectratio]{images/bias_fit_BOOSTCOV.pdf}
	\includegraphics[width=.49\linewidth, keepaspectratio]{images/RH_vs_z_diff_0_10.pdf}		
	\caption{\label{fig:Rh_z_effDiff} 
	Left: Boosting factor on the error in the correlation function. 
	Right: $R_H^{D_2=2.97}(z)$ with (circle) and without (triangle) boosting the errors, for NGC (red) and SGC (blue).}
\end{figure}

The theoretical model for redshift space distorsions (Eq.~\ref{eq:LSS_RSD}) is not perfectly accurate at the smallest scales due to the real nonlinear behaviour of gravity at these scales. In order to ensure satisfying $\chi^2/$n.d.f.\ for the RSD fitting,
we boost the error on $\xi(r)$ at the relevant scales in an empirical way as
\begin{equation}
		C^{'}_{ij} = C_{ij} ( 1 + \delta_{ij}\Delta_{i}\Delta_{j}e^2 ) \; .
\end{equation}
Here $\delta_{ij}$ is the usual Kronecker symbol; $e$ is a parameter that measures the amount of error boosting we apply; $\Delta_{i}$ is the theoretical inaccuracy, estimated as the relative difference between our model and the average of the $1000$ QPM mock catalogues. Figure \ref{fig:Rh_z_effDiff} (left) presents the resulting boosting factor on the error in the correlation function. It appears to be significant only on scales smaller than 10 $h^{-1}$ Mpc.
Fig.~\ref{fig:Rh_z_effDiff} (right) shows that the reconstructed homogeneity scales measured with $\mathcal D_2$ is not significantly modified by the error boosting.

%------------------------------------------------------------------------------------------------------------------------
\section{Test of spline fit on QPM mock catalogues}\label{subsec:Robustness}  	
 
We perform a spline fit of $\mathcal{D}_2$ for the 1000 QPM mock catalogues in order to obtain the homogeneity scale at 1\% (Eq. \ref{eq:RH-definition}). 
The fit is performed in the range $r \in [40,100]\ h^{-1}$ Mpc with $6$ data points and $1$ degree of freedom. The distribution of the $\chi^{2}$ of the mock should therefore follow a $\chi^{2}$-law for 1 degree of freedom. In table (\ref{tab:chi2Splines}) we show the mean and the error on the mean of the distribution of the corresponding $\chi^2$ for the $1000$ QPM mock catalogues. The test is successful in both NGC and SGC.

\begin{table}[h!]
		\begin{center} 
		\begin{tabular}{ *3c } 
	 	$z$   & $\chi^2_{\rm NGC}$ & $\chi^2_{\rm SGC}$  \\ 
	 	\hline 
		0.430-0.484 & $1.00\pm0.05$  & $0.99\pm0.04$   \\ 
	 	0.484-0.538 & $0.99\pm0.05$  & $1.00\pm0.04$   \\ 
	 	0.538-0.592 & $1.02\pm0.05$  & $1.00\pm0.04$   \\ 
		0.592-0.646 & $0.99\pm0.04$  & $1.00\pm0.05$   \\ 
		0.646-0.700 & $1.02\pm0.05$  & $1.00\pm0.04$   \\  
	 	\hline
		\end{tabular}
		\end{center} 
\caption{\label{tab:chi2Splines} Mean and error over the $1000$ QPM mock catalogues for the $\chi^2$ of the spline fit with 1 degree of freedom, in the NGC and SGC for the five redshift bins.}
\end{table}	
	
%\newpage
%------------------------------------------------------------------------------------------------------------------------
\section{Homogeneity scale at 0.1\%}

The choice of a 1\% threshold to define the homogeneity scales is arbitrary. We can define them for instance at 0.1\% as:
	\begin{equation}\label{eq:RH-definition1}
		\mathcal{D}_{2}(R^{\mathcal{D}_2=2.997}_H) = 2.997 \quad {\rm or} \quad \mathcal{N}(R^{\mathcal{N}=1.001}_{H}) = 1.001
	\end{equation}
Figure \ref{fig:RH-z-perMil} shows that the measured homogeneity scale for matter distribution is compatible with $\Lambda$CDM, with 
$\chi_{red}^{2} =5.82/6$ in the NGC and $\chi_{red}^{2} = 7.98/6$ in the SGC.
	
\begin{figure}[h!]
	\centering
	\includegraphics[width=100mm]{images/RH_z_QPMErr_perMil_QSO.pdf}
	\caption{\label{fig:RH-z-perMil} The homogeneity scale at 0.1\% level, $R^{\mathcal{D}_2=2.997}_H(z)$, measured in the NGC (red) and in the SGC (blue) as a function of redshift. The purple point is the result obtained with quasars in the NGC,  in the redshift range $2.2\le z \le 2.8$ by \citet{Laurent}.
	The green line is the $\Lambda$CDM model prediction. The shaded areas indicate the 1$\sigma$ range for the 1000 QPM mock catalogues.}	
\end{figure}
